# Supplementary material for: Droplet splashing during the impact on liquid pools of shear-thinning fluids with yield stress
Source: arXiv:2110.09328 source file (2021-10-18)
Supplement: Supplementary file 1 [file NonNewtonianDropletImpact-SM.pdf]

# Droplet splashing during the impact on liquid pools of shear-thinning fluids with yield stress: Supplementary material

Xiaoyun Peng (彭小芸),[1] Tianyou Wang (王天友),[1] Kai Sun (孙凯),[1] and Zhizhao Che (车志钊)[1, a)]

*State Key Laboratory of Engines, Tianjin University, Tianjin, 300072, China.*

(Dated: 18 October 2021)

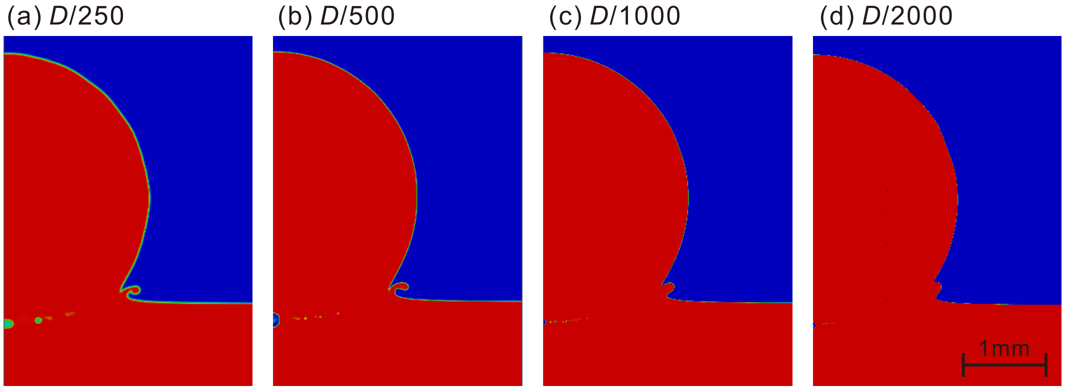


FIG. S1. Mesh independency study. Simulations were performed by progressively refining the mesh with the same physical parameters. The smallest cell is changed from $D/250$, $D/500$, $D/1000$ to $D/2000$, and the snapshots are at the dimensionless time of 0.09, Re = 187.59, and We = 220.94.

[a)]Electronic mail: chezhizhao@tju.edu.cn

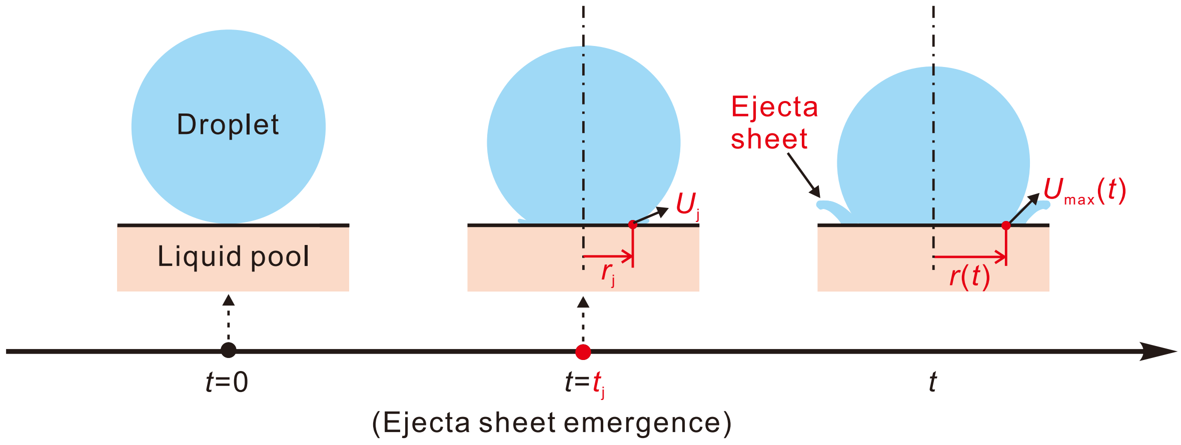


FIG. S2. Schematic diagram of ejecta sheet emergence. $r(t)$ is the spreading radius, $U_{\max}(t)$ is the maximum velocity in the liquid above the initial surface plane of the liquid pool, $r_{\mathrm{j}}$ is the spreading radius of ejecta sheet emergence, $U_{\mathrm{j}}$ is the velocity of ejecta sheet emergence, and $t_{\mathrm{j}}$ is the time of ejecta sheet emergence.

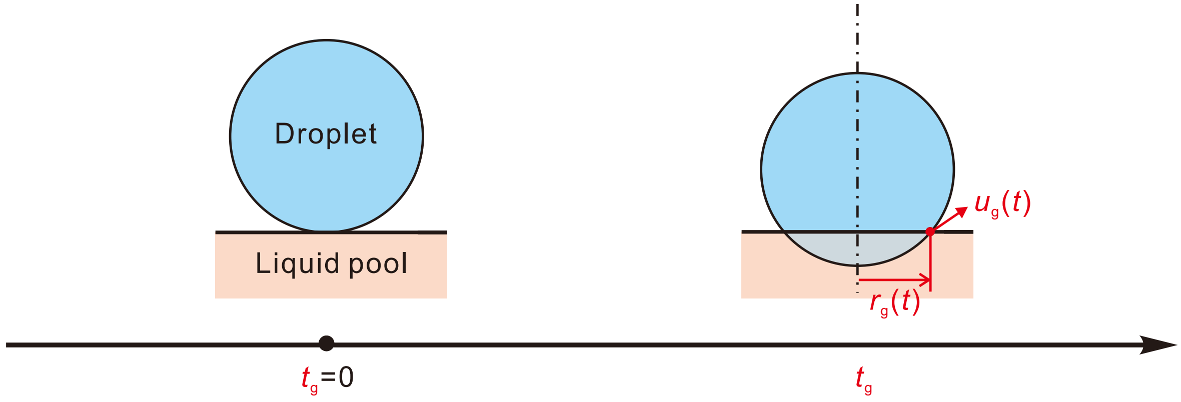


FIG. S3. Schematic diagram of geometrical law. $r_{\mathrm{g}}(t)$ is the geometrical law for the spreading radius, $u_{\mathrm{g}}(t)$ is the geometrical velocity, and $t_{\mathrm{g}}$ is the geometrical time.

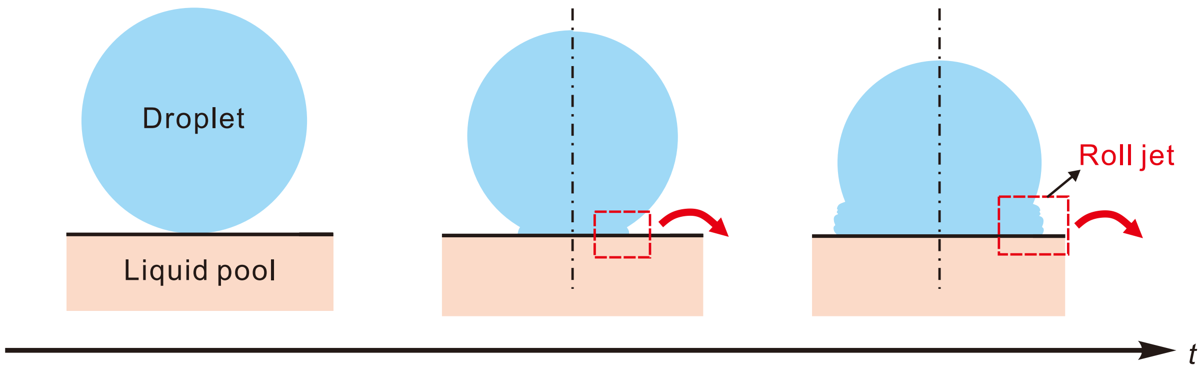


FIG. S4. Schematic diagram of the roll jet emergence.
